# Supplementary material for: Quantization of mode shifts in nanocavities integrated with atomically thin sheets
Source: arXiv:2201.06684 source file (2022-01-18)
Supplement: Supplementary file 1 [file 2DXcavity-SI.pdf]

**Supplementary Information**

# Quantization of mode shifts in nanocavities integrated with atomically thin sheets

Nan Fang[1], Daiki Yamashita[2], Shun Fujii[2], Keigo Otsuka[1,3], Takashi Taniguchi[4], Kenji Watanabe[5], Kosuke Nagashio[6], Yuichiro K. Kato[1,2]

[1]Nanoscale Quantum Photonics Laboratory, RIKEN Cluster for Pioneering Research, Saitama 351-0198, Japan

[2]Quantum Optoelectronics Research Team, RIKEN Center for Advanced Photonics, Saitama 351-0198, Japan

[3]Department of Mechanical Engineering, The University of Tokyo, Tokyo 113-8656, Japan

[4]International Center for Materials Nanoarchitectonics, National Institute for Materials Science, Ibaraki 305-0044, Japan

[5]Research Center for Functional Materials, National Institute for Materials Science, Ibaraki 305-0044, Japan

[6]Department of Materials Engineering, The University of Tokyo, Tokyo 113-8656, Japan

These authors contributed equally: Nan Fang, Daiki Yamashita.

# Supplementary Note 1:

## Spatial profiles of the modes in air- and dielectric-mode cavities.

We use finite-difference time-domain (FDTD) simulation to calculate the mode profiles in different cavities. In Fig. 1 (c, d), we have shown that the spatial distribution of the *y*-component of the electric field $E_y$ at different views for both air-mode and dielectric-mode cavities. To compare the evanescent fields more clearly, we plot $E_y^2$ along the *z* direction from the cavity center. As indicated in Supplementary Fig. 1, the relative intensity of the evanescent fields of the air mode is much larger than that in the dielectric mode. Since 2D materials are transferred above the cavity, the use of the air-mode cavity should be beneficial for the enhanced coupling with the 2D materials.

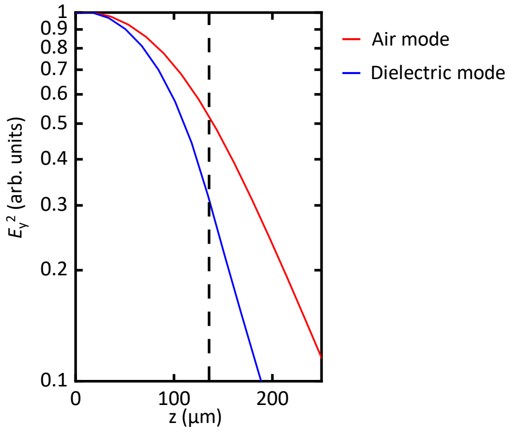


**Supplementary Fig. 1 | Evanescent fields in different cavities.** The calculated normalized spatial distribution of $E_y^2$ for the fundamental transverse-electric mode along the *z* direction. Red and blue lines represent air and dielectric modes, respectively. The coordinate origin is taken to be the center of the cavity, and the dashed line indicates the surfaces of the different cavities.

# Supplementary Note 2:

## Environmental effect on cavity modes

We observe that the resonant modes are sensitive to the measurement environment in some nanobeam cavities that are integrated with tungsten diselenide ($WSe_2$) flakes. As shown in the photoluminescence (PL) spectra of Supplementary Fig. 2a, the peak of the cavity mode measured in ambient air is redshifted and broadened compared to that measured in dry nitrogen gas. Our air-mode nanobeam cavities have large evanescent fields and could be sensitive to the adsorption of water molecules by $WSe_2$ in ambient air. In comparison, the bare nanobeam cavity mode is insensitive to the measurement environment (Supplementary Fig. 2b). We therefore measure all the cavities in dry nitrogen gas to eliminate the environmental effect.

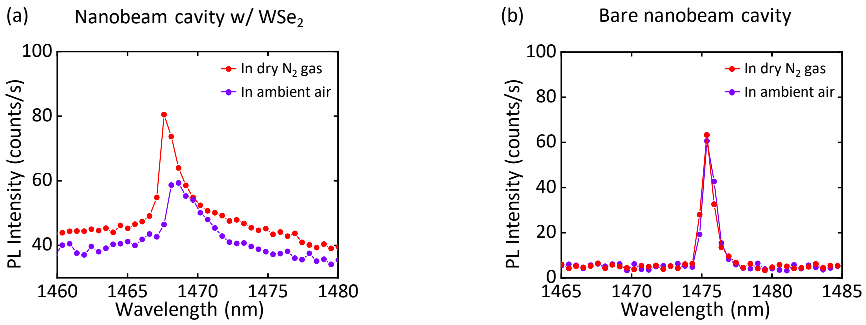


**Supplementary Fig. 2 | Influence of the environment on cavity modes. a**, PL spectra of the fundamental mode for an air-mode nanobeam with a thin $WSe_2$ flake (< 4 layers) on top measured in ambient air (purple) and dry nitrogen gas (red). **b**, PL spectra of the fundamental mode for a bare air-mode nanobeam measured in ambient air (purple) and dry nitrogen gas (red). The excitation power is 300 $\mu$W and the excitation wavelength is 780 nm.

# Supplementary Note 3:

## Wavelength shifts in high-order modes

The fabricated nanobeam cavities have several modes from the fundamental one (zeroth) to high-order ones (first and second). High-order modes appear at the longer wavelength region for the dielectric mode and the shorter wavelength region for the air mode. Supplementary Fig. 3a shows PL spectra of a dielectric-mode nanobeam cavity before and after the transfer of a 9.0-nm-thick $WSe_2$ flake. The wavelength shifts are dependent on the orders of the mode, and higher-order ones have larger shift values (Supplementary Fig. 3b). We apply FDTD calculations to simulate the spatial distribution of $E_y$ for the different modes (Supplementary Fig. 3c-e). High-order modes have larger mode volumes that interact with the $WSe_2$ flake, which explains the greater shifts here.

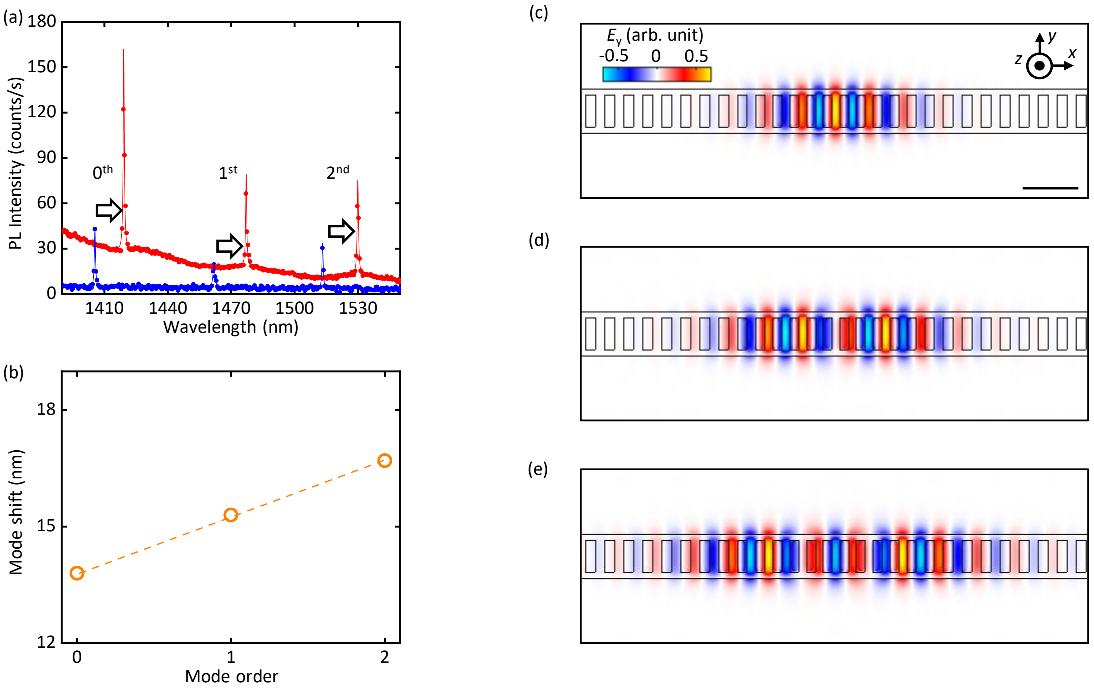


**Supplementary Fig. 3 | Mode order dependence of wavelength shifts a**, PL spectra for a dielectric-mode nanobeam before (blue) and after (red) the transfer of a 9.0-nm-thick $WSe_2$ flake. The excitation power is 300 $\mu$W and the excitation wavelength is 780 nm. **b**, Resonant wavelength shifts for different modes. Calculated spatial distribution of $E_y$ for the mode of zeroth (**c**), first (**d**), and second order (**e**), respectively. The scale bar is 1 $\mu$m.

# Supplementary Note 4:

## Air-space effect on resonant wavelength shifts

In addition to Fig. 3 in the main text, we perform atomic force microscopy (AFM) for two $WSe_2$/cavity samples with different $WSe_2$ thickness. In Supplementary Fig. 4a, the 44-nm-thick $WSe_2$ flake has a uniform morphology over trenches. In comparison, a clear air space appears between the 15-nm-thick $WSe_2$ flake and the cavity as shown in Supplementary Fig. 4b. From the measured ten samples, we observe that most of the samples with thin $WSe_2$ flakes of the thickness < 20 nm have the air space of about 10-30 nm. The air space is thought to form when peeling off the PDMS stamp from the substrate with trenches. The region of the $WSe_2$ flake just above the trench is pulled up because the thin samples are easily deformed under external strains. We then simulate the air-space effect on the mode shifts by using FDTD simulation, and the sample geometry is indicated in Supplementary Fig. 4c. Supplementary Fig. 4d shows that the $WSe_2$-induced redshift is reduced from 60.2 to 34.5 nm when the distance of the air space reaches 40 nm. The decreased shifts are due to the weakening of the coupling between the 2D material and the cavity mode.

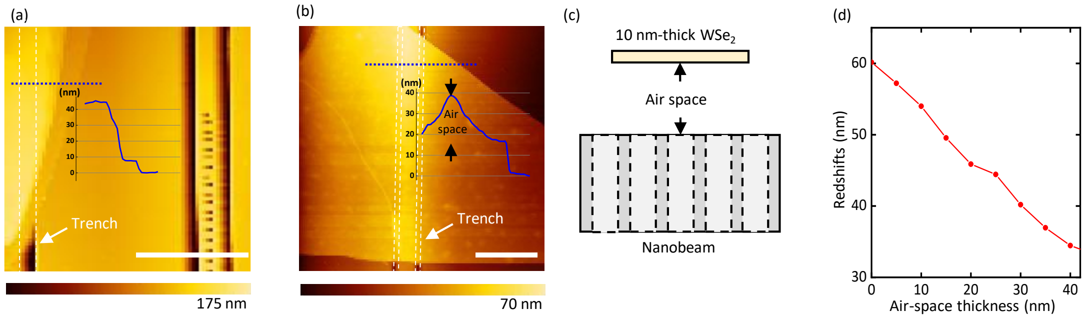


**Supplementary Fig. 4 | Air space between 2D materials and trenches. a,** An AFM image of the 44-nm-thick $WSe_2$/nanobeam hybrid. **b**, An AFM image of the 15-nm-thick $WSe_2$/nanobeam hybrid. The scale bars are 5 $\mu$m. The inset is the height profile indicated by the broken line (blue). **c**, The model for the simulation of the air-space effect. 2D material here is $WSe_2$ with dielectric constant $\varepsilon$ = 19 and thickness = 15 nm. **d**, Simulated air-space distance dependence of the redshifts.

# Supplementary Note 5:

## Dielectric constant dependence of the resonant wavelength shifts

It is known that different types of 2D materials have various dielectric constant $\varepsilon$ [1]. We perform FDTD calculations to simulate the $\varepsilon$ dependence of the cavity mode resonant wavelength shifts. In the simulation, a 2D material flake is placed above an air-mode cavity and the wavelength shifts are calculated at different in-plane $\varepsilon$ of the 2D material. The thickness of the 2D flake is defined as 11.6 nm, which is the average thickness of the four flakes in Fig. 2 of the main text. As indicated in Supplementary Fig. 5, the shifts are linearly dependent on the dielectric constant when $\varepsilon < 20$ and show superlinear behavior when $\varepsilon > 20$. Such a strong dielectric constant dependence explains various wavelength tuning capabilities of the different 2D materials as shown in the main text of Fig. 2. We also simulate the out-of-plane $\varepsilon$ dependence, and find that out-of-plane $\varepsilon$ has little effect on the redshifts of the cavity mode.

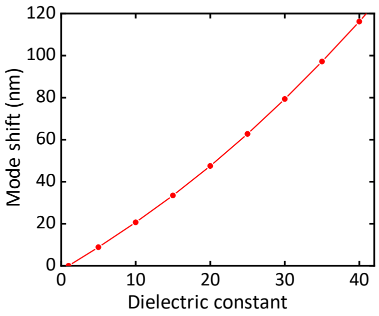


**Supplementary Fig. 5 | Dielectric constant dependence of resonant wavelength shifts.** Simulated in-plane dielectric constant dependence of the mode shifts.

# Supplementary Note 6:

## Transmittance measurements of $WSe_2$/cavity hybrid

We perform the transmittance measurement to detect the cavity *Q* factor by using a dimpled tapered nanofiber with the following processes [2]. We first fabricate a tapered fiber by heating and pulling a standard single-mode optical fiber. We then prepare another bare optical fiber and bring it into contact with the tapered fiber, followed by the heating at the contact area to form a dimple in the nanofiber. The bent and tensed fiber can be positioned close to the top of the cavity, enabling the coupling of light from the fiber into the nanobeam cavity. The transmittance spectrum for a bare nanobeam cavity is recorded when the dimpled fiber is in contact (Supplementary Fig. 6a). The fundamental cavity mode is observed as the dip with the resonant wavelength of ~ 1425.79 nm and the *Q* factor of ~22490. We then transfer a 22.0 nm-thick $WSe_2$ flake on top of the cavity, and the corresponding transmittance spectrum is shown in Supplementary Fig. 6b. The resonant wavelength is redshifted to ~ 1537.44 nm, and the *Q* factor is ~ 22780. We note that *Q* factor measured here is in the under-coupled condition, which reveals the intrinsic value of the cavity [3]. It is surprising to observe that the *Q* factor essentially remains the same despite the large wavelength shift, indicating a clean transfer process as well as the absence of the absorption from the $WSe_2$ flake. The resonant modes in the thicker $WSe_2$/cavity hybrids could not be observed by the transmittance measurement, possibly due to a severe modification of the evanescent field profile by the $WSe_2$ flake. We also simulate the *Q* factor as a function of the $WSe_2$ thickness by FDTD calculations (Supplementary Fig. 6c). *Q* factor shows a slight decrease in thin $WSe_2$ samples and remains almost unchanged in the range of 15-45 nm.

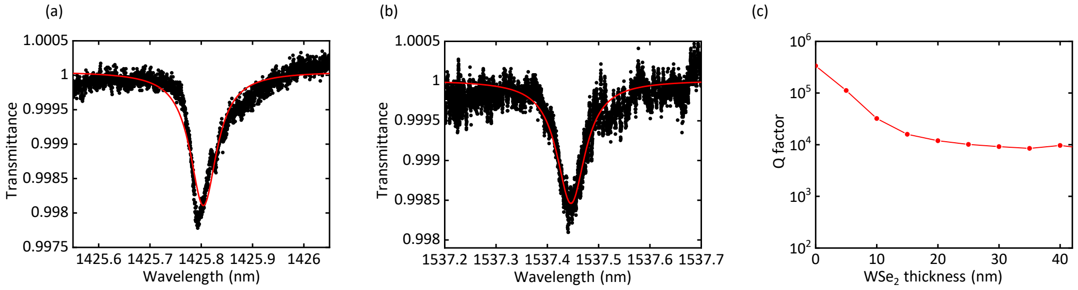


**Supplementary Fig. 6 | Q factor evaluation of the $WSe_2$/nanobeam hybrid by transmittance measurement. a**, Transmittance spectrum of a tapered fiber coupled with the bare nanobeam cavity. The vertical axis is normalized with the maximum transmittance of the tapered fiber. **b**, Transmittance spectrum of the tapered fiber coupled with the 22.0 nm-thick $WSe_2$/nanobeam hybrid. Dots are data and solid lines are Lorentzian peak fits. **c**, Calculated Q factor as a function of $WSe_2$ thickness by FDTD simulation.

## Supplementary Note 7:

### Procedure for anthracene-assisted dry transfer

Supplementary Fig. 7a-f illustrate the transfer procedure of the 2D flake using an anthracene stamp [4]. The anthracene single crystal is picked up with a glass-supported PDMS sheet to form the anthracene/PDMS stamp. 2D flakes are prepared on a standard 90-nm-thick $SiO_2$/Si substrate by mechanical exfoliation, and their layer number is determined by the optical contrast. The target 2D flake is picked up by pressing the anthracene/PDMS stamp against the substrate for 5 min, followed by the quick separation (> 10 mm/s) so that the anthracene crystal remains attached to the PDMS sheet. The stamp is then pressed on a receiving substrate for 5 min. By slowly peeling off the PDMS (< 0.2 $\mu$m/s), the anthracene crystal with the target 2D flake is released on the substrate. Sublimation of the anthracene in the air leaves behind clean 2D flakes on any substrate because contamination from solvents is absent in the all-dry process. Supplementary Fig. 7g and h show the optical micrographs of a molybdenum sulfide ($MoS_2$) flake before and after the transfer. A clean surface is observed, which is confirmed by the AFM image (Supplementary Fig. 7i).

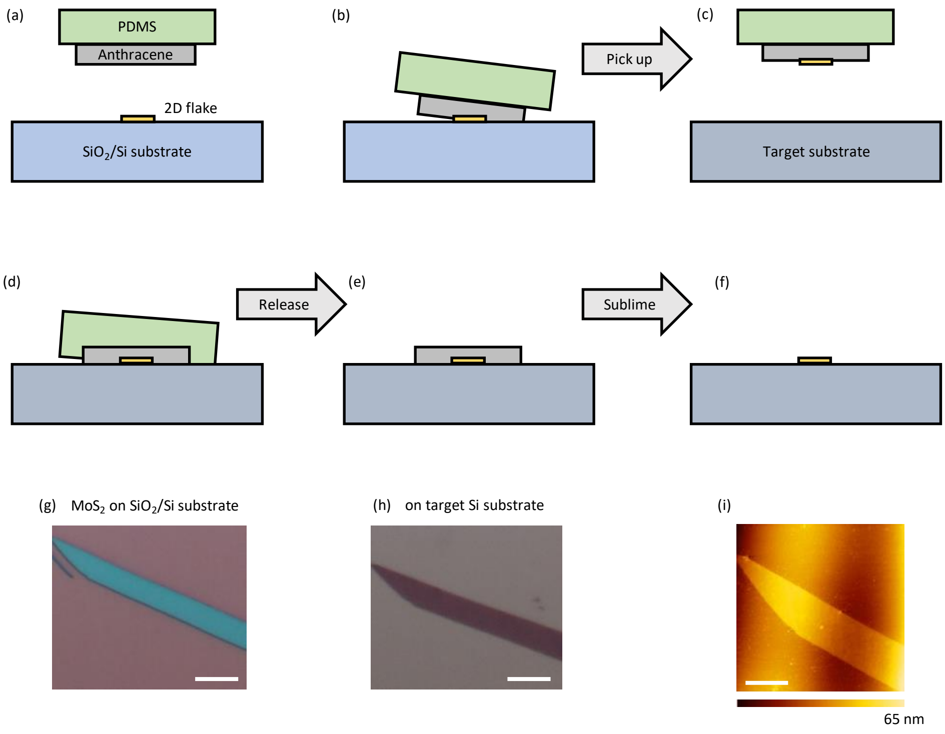

**Supplementary Fig. 7 | Anthracene-assisted dry transfer process. a**, 2D flakes prepared on a standard 90-nm-thick $SiO_2$/Si substrate by mechanical exfoliation, and an anthracene single crystal is picked up with a glass-supported PDMS sheet to form an anthracene/PDMS stamp. **b**, Press the anthracene/PDMS stamp against the substrate on the target flake position for 5 min. Half of the anthracene/PDMS stamp does not contact the substrate to prevent the anthracene crystal from falling down to the substrate. **c**, 2D flakes are picked up by quick separation of > 10 mm/s. **d**, The stamp is pressed on a receiving substrate with submicron position control. **e**, The anthracene crystal with the target 2D flake is released on the substrate by slowing peeling off the PDMS (< 0.2 $\mu$m/s). **f**, The anthracene crystal is sublimated in the air at 110 °C for 10 min. Optical micrographs of a $MoS_2$ flake (**g**) before and (**h**) after the transfer on the different substrates. (**i**) An AFM image of the $MoS_2$ flake after the transfer. The scale bars in g, h, i are 10, 10, and 5 $\mu$m, respectively.

# Supplementary Note 8:

## Selective pick-up of 2D flakes by anthracene crystals

Unlike the PDMS stamp, the anthracene stamp is capable of picking up 2D flakes and is used to demonstrate the reversible control of 2D/cavity hybrids as shown in Fig. 5. Here we investigate the pick-up process of various 2D materials by the anthracene stamp, and the pick-up probability is defined as the number of the picked-up 2D flakes over the total number of the contacted flakes. Supplementary Fig. 8a shows an optical image with an anthracene crystal attached to a $SiO_2$/Si substrate, and six 2D flakes are contacted. After the quick separation from the substrate, three out of six flakes are attached to the anthracene stamp (Supplementary Fig. 8b), and therefore, the pick-up probability is 50%. We have tried different types of 2D flakes, and pick-up probability is summarized in Supplementary Fig. 8c. We find that *p*-$MoS_2$ and graphene are very difficult to be picked up, while *n*-$MoS_2$, $WSe_2$, and hexagonal boron nitride (h-BN) flakes are easily picked up with an average probability of ~50%. The selectivity of the pick-up process may come from the electrostatic force because different types of 2D materials have different carrier types and densities [5]. We note that the pick-up probability of carbon nanotubes by the anthracene stamp is less than 1% [4] and is much smaller than that for *n*-$MoS_2$, $WSe_2$, and h-BN. Such a large contrast in the pick-up probability indicates a stronger interaction between the 2D materials and anthracene crystals.

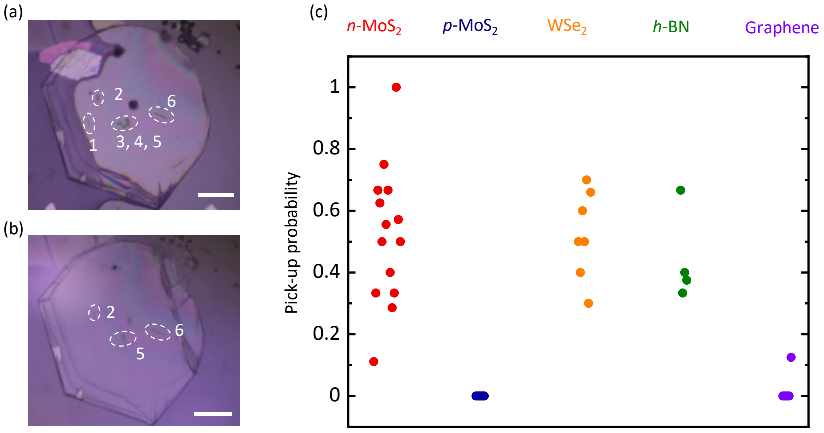


**Supplementary Fig. 8 | Pick-up probability for different types of 2D materials.** Optical micrographs of the anthracene (**a**) when contacting with, (**b**) after separation from the substrate. Circles indicate the 2D flakes adhering to the anthracene crystal. Scale bars are 150 $\mu$m. **c,** Pick-up probabilities for different types of 2D materials.

## Supplementary Note 9:

## PL spectra of 2D materials by anthracene-assisted dry transfer method

To demonstrate the versatility as well as the minimal perturbation of the anthracene-assisted dry transfer method, we have prepared the monolayer $MoS_2$ flake on different substrates and the representative PL spectra are indicated in Supplementary Fig. 9a. The PL spectrum from the suspended monolayer $MoS_2$ has one main narrow exciton peak with the width of ~ 21.2 nm, suggesting the minimal doping effect after the sublimation of the anthracene [6]. In comparison, the PL spectrum from $SiO_2$/Si substrate shows the much broader peak. We also use this transfer method to prepare the heterostructure that consists of a monolayer $MoS_2$ flake on a bulk h-BN flake. The PL spectrum from the heterostructure is comparable with that from the suspended $MoS_2$, indicating the superior interfacial property between h-BN and $WSe_2$. The PL spectroscopy is also performed for the monolayer $WSe_2$/nanobeam hybrid in Fig. 4a of the main text, and the spectrum is indicated in Supplementary Fig. 9b. Monolayer $WSe_2$ on the cavity holes shows higher peak intensity than that on the substrate, which could be explained by the reduced quenching effect from the substrate with many air holes. Moreover, no obvious change in the spectral line shape is observed, indicating a minimal strain in $WSe_2$/nanobeam hybrids [7].

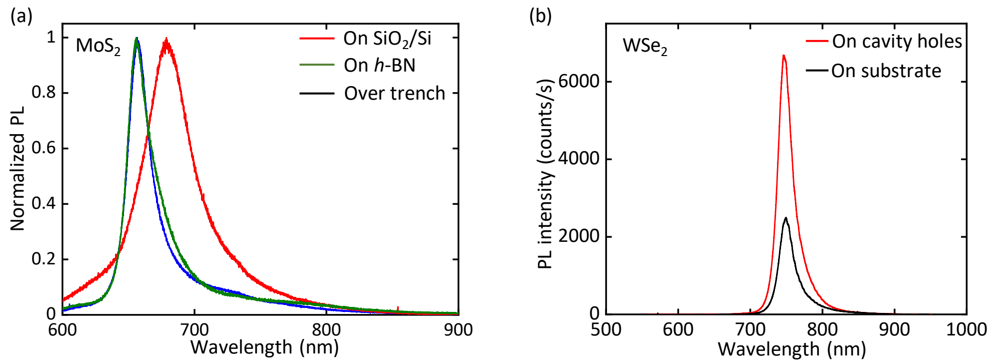


**Supplementary Fig. 9 | PL spectra to evaluate the anthracene-assisted dry transfer method. a**, PL spectra of monolayer $MoS_2$ flakes on the $SiO_2$/Si substrate (red), on the h-BN flake (green), and over the trench (blue). **b**, PL spectra of monolayer $WSe_2$ flakes on cavity holes (red) and on the substrate (black). The excitation wavelength is 488 nm, and the power is 1.5 $\mu$W.

**REFERENCES**

S1. Laturia, A. *et al.* Dielectric properties of hexagonal boron nitride and transition metal dichalcogenides: from monolayer to bulk. *npj 2D Mater. and Appl.* **2**, 1-7 (2018).

S2. McCutcheon, M. W. *et al.* High-Q transverse-electric/transverse-magnetic photonic crystal nanobeam cavities, *Appl. Phys. Lett.* **98**, 111117 (2011).

S3. Tetsumoto, T. *et al.* High-Q coupled resonances on a PhC waveguide using a tapered nanofiber with high coupling efficiency. *Opt. express* **23**, 16256-16263 (2015).

S4. Otsuka, K. *et al*. Deterministic transfer of optical-quality carbon nanotubes for atomically defined technology. *Nat. commun.* **12**, 3138 (2021).

S5. Fang, N. *et al.* Full Energy Spectra of Interface State Densities for n - and p - type MoS2 Field - Effect Transistors. *Adv. Funct. Mater.* **29**, 1904465 (2019).

S6. Yu, Y. *et al.* Engineering substrate interactions for high luminescence efficiency of transition - metal dichalcogenide monolayers. *Adv. Funct. Mater.* **26**, 4733-4739 (2016).

S7. Desai, S. *et al.* Strain-induced indirect to direct bandgap transition in multilayer $WSe_2$. *Nano Lett.*, **14**, 4592-4597 (2014).
